# Supplementary material for: Robust and Performance Incentivizing Algorithms for Multi-Armed Bandits with Strategic Agents
Source: arXiv:2312.07929 source file (2025-03-09)
Supplement: Supplementary file 1 [file some_facts_appendix.tex]

\section{Some Facts}
\begin{lemma}\label{app:hetro_sub_bound}
Given that an arm $j\in \armstop$ follows the best performance strategy of giving $\maxall$, then for any arm $i \in \arms-\armstop$ we have $\E[T_{i}(n)] \leq \frac{2 \ln(n)}{(\maxall-M_{i})^2} = o(n)$.
\end{lemma}
\begin{proof}
Let $j$ be an arm in $\armstop$ then arm $j$ always outputs a reward of $\maxall$, further arm $i$ can at most give a reward of $M_{i} < \maxall$, therefore we have: 
\begin{align}
    \E[T_{i}(n)] & \leq \E\Big[\sum_{t=1}^n  \indic[I_t=i , T_{i}(t-1) \leq \frac{2 \ln(n)}{(\maxall-M_{i})^2}] \\ 
    & \sum_{t=1}^n \indic[I_t=i , T_{i}(t-1) > \frac{2 \ln(n)}{(\maxall-M_{i})^2} ]\Big] \\  
    & \leq \frac{2 \ln(n)}{(\maxall-M_{i})^2} + \sum_{t=1+\frac{2 \ln(n)}{(\maxall-M_{i})^2}}^n \Pr\Big(UCB_{i}(t-1) \ge UCB_{j}(t-1), T_{i}(t-1) > \frac{2 \ln(n)}{(\maxall-M_{i})^2}\Big)
\end{align}
But we can bound $UCB_{i'}(t-1)$ by the following:
\begin{align}
     UCB_{i}(t-1) & \leq M_{i} + \sqrt{\frac{2\ln(n)}{T_{i'}(t-1)}} \\ 
     & < M_{i} + \sqrt{\frac{2\ln(n)}{\frac{2 \ln(n)}{(\maxall-M_{i})^2}}} && (\text{if $T_{i}(t-1) > \frac{2 \ln(n)}{(\maxall-M_{i})^2}$})\\ 
     & = \maxall \leq UCB_{j}(t-1)
\end{align}
Therefore $\Pr\Big(UCB_{i}(t-1) \ge UCB_{j}(t-1), T_{i}(t-1) > \frac{2 \ln(n)}{(\maxall-M_{i})^2}\Big)=0$ and $\E[T_{i}(n)] \leq \frac{2 \ln(n)}{(\maxall-M_{i})^2}=o(n)$. 
\end{proof}
